# Supplementary material for: Local characterization of hindered Brownian motion by using digital video microscopy and 3D particle tracking
Source: arXiv:1408.4309 source file (2014-08-19)
Supplement: Supplementary file 1 [file supplementary.pdf]

# Local characterization of hindered Brownian motion by using digital video microscopy and 3D particle tracking: Supplemental Information

Simon L Dettmer,[1] Ulrich F Keyser,[1] and Stefano Pagliara[1]
*Cavendish Laboratory, University of Cambridge, 19 J J Thomson Avenue, Cambridge, CB3 0HE, United Kingdom*

(Dated: 25 January 2014)

In this supplementary we consider the possibility that particles get mixed up when linking the positions into trajectories. We remind the reader that the linking process was solved locally by placing boxes around the particle centers from the previous frame and then looking for location candidates only within that box. As long as there is only one particle inside the box, the positions of different particles cannot be swapped in between frames. If a second particle is present inside the box, the one closest to the box center is chosen as the next position in the trajectory. We now ask ourselves:

1. How likely is it to have more than one particle in the tracking box?
2. What is the probability of the two particles being mixed up in the linking process?

## I. PROBABILITY TO HAVE MORE THAN ONE PARTICLE INSIDE THE BOX

Let us assume that we have $N$ particles moving independently in the total system volume. Then, assuming the particle is to be in any place with equal probability, the probability to find a fixed particle inside the tracking box is simply the ratio of volume of that box to the total system volume $p = V_{box}/V_{tot}$ (For colloids with close to neutral buoyancy, which is the case for our experiment, we can neglect particle depletion at the top of the microfluidic chip). From the independence assumption follows that the number $K$ of particles inside the box is binomially distributed:

$$P(K=n) = \mathcal{B}_{N,p}(n) = p^n(1-p)^{N-n}\binom{N}{n} \qquad (1)$$

In the limit of large particle number, $N \gg 1$, this converges to the Poisson distribution:

$$\begin{aligned} P(K=n) = \mathcal{P}_{Np}(n) &= \frac{(V_{box}\frac{N}{V_{tot}})^n}{n!}e^{-V_{box}\frac{N}{V_{tot}}} \\ &= \frac{(V_{box}c)^n}{n!}e^{-V_{box}c} \qquad (2) \end{aligned}$$

where we have inserted the particle concentration $c = N/V_{tot}$. Since we only have a tracking box if there is at least one particle, we have to condition the probability on the event that there is at least one particle inside the box. In total we get:

$$P_{>2box} = \frac{P(n\geq 2)}{P(n\geq 1)} = 1 - V_{box}c\frac{e^{-V_{box}c}}{1-e^{-V_{box}c}} \qquad (3)$$

In our experiment we used a particle concentration of $c = 0.1\ \mu m^{-3}$ and a tracking box size of $30 \times 30\ px^2$. With an approximate tracking depth of 2 $\mu m$ we arrive at a box volume of $V_{box} = 7.34\ \mu m^3$ and thus a probability to have more than one particle inside the tracking box of 32 %.

## II. PROBABILITY OF CONFUSING PARTICLES IN THE LINKING PROCESS

We will now show that the probability of mixing-up-events is quite low and an upper bound can be given independent of the box size used.

Let us consider two colloids of radius $a$ inside the tracking box, undergoing 2D-Brownian motion with diffusivity $D$. At time $t = 0$ the box is centered on the position of colloid 1 (Figure S.1a)). We will choose the origin of our coordinate system to coincide with the box center. Let us denote the positions of the colloids by $r_1(t)$ and $r_2(t)$. Then we have $\vec{r}_1(0) = 0$ and without loss of generality we can assume $\vec{r}_2(0) = r_0\vec{e}_x$ with $r_0 \geq 2a$ enforced by the fact that particles cannot intersect each other. Nonetheless, for simplifying the calculations (and making them at all possible) we will assume for the following particle motion that the colloids can intersect each other. It is obvious that doing this can only increase the probability of mixing up particles since the proper colloid 1 loses the option of protecting the center of the box by pushing away the other colloid. Now the criterion for mixing up particles in the next frame (Figure S.1b)) is that at time $t = \tau$, colloid 2 is closer to the center than colloid 1, i.e. $r_1^2(\tau) > r_2^2(\tau)$. Therefore the probability of mixing up particles has an upper bound given by:

$$P_{mix} = \int_0^\infty p(r_1^2(\tau) > r_2^2(\tau)|r_2^2(\tau)=z)p(r_2^2(\tau)=z)dz \qquad (4)$$

The first probability density in (4) is obviously given by

$$\begin{aligned} p(r_1^2(\tau) > r_2^2(\tau)|r_2^2(\tau)=z) &= \int_z^\infty p(r_1^2(\tau)=y)dy \\ &= \int_z^\infty \frac{1}{4D\tau}e^{-\frac{y}{4D\tau}}dy \\ &= e^{-\frac{z}{4D\tau}} \qquad (5) \end{aligned}$$

where we used the widely known propagator of Brownian motion as well as its convolution for the probability density of $r_1^2(\tau)$ (see e.g. Qian et al.[1]).

The second density in (4) can similarly be derived from the diffusion propagator and is given by:

$$\begin{aligned} p(r_2^2(\tau)=z) &= \frac{1}{2\sqrt{z}} p\left(|\vec{r}_2(\tau)| = \sqrt{z}\right) \\ &= \frac{1}{2\sqrt{z}} \int_{-\sqrt{z}}^{\sqrt{z}} p\left(\begin{pmatrix} x_2(\tau) \\ y_2(\tau) \end{pmatrix} = \begin{pmatrix} \xi \\ \pm\sqrt{z-\xi^2} \end{pmatrix}\right) d\xi \\ &= \frac{1}{\sqrt{z}} \int_{-\sqrt{z}}^{\sqrt{z}} \frac{1}{4\pi D\tau} e^{-\frac{(\xi-r_0)^2}{4D\tau} - \frac{z-\xi^2}{4D\tau}} d\xi \\ &= \frac{1}{\pi r_0 \sqrt{z}} e^{-\frac{r_0^2+z}{4D\tau}} \sinh\left(\frac{2r_0\sqrt{z}}{4D\tau}\right) \end{aligned} \quad (6)$$

Inserting (5) and (6) into (4) we do not find a direct expression for the probability but we can numerically solve the integral for the values concerned. Naturally, the probability to mix up the particles must increase with decreasing separation. This manifests itself in the $\exp(-r_0^2/4D\tau)$ term in (6). Therefore to obtain an upper bound we use the smallest possible distance, $r_0 = 2a = 505$ $nm$, i.e. touching colloids. Making a conservative estimate for the diffusivity, $D = 0.8\mu m^2/s$ and using the inter-frame-time $\tau = 33$ $ms$ we find $P_{mix} = 0.069$, i.e. in less than 7 % of the cases where two particles are present inside the box, they get swapped in the linking process. Typical frequencies of these events will be a lot smaller due to the second colloid generally being further away than $2a$ and the impossibility of intersecting particles. Interestingly this estimate is independent of the box size used and shows that the chosen linking algorithm should perform well even at extremely high particle concentrations.

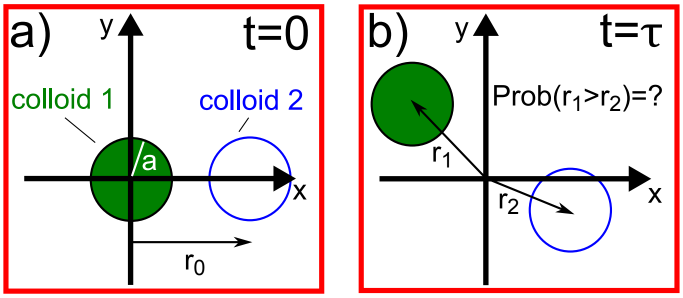


FIG. S.1. Schematic view of mixing up particles in the tracking box. a) At $t = 0$ the tracking box (red line) is centered on the first (proper) colloid. Additionally, there is a second colloid present at a distance $r_0$. b) At the next video frame ($t = \tau$), both particles have diffused away from their original positions. Since the particle closest to the box center is linked to the position of colloid 1 at $t = 0$, swapping of particles occurs if the second colloid is closer than the first one, i.e. $r_1 > r_2$.

[1] H. Qian, M. Sheetz, and E. Elson, Biophysical Journal **60**, 910 (1991).
